# Supplementary material for: From Evaluation to Enhancement: Benchmarking and Improving Think-with-Video Reasoning for Video Generative Models
Source: arXiv:2609.11242 source file (2026-09-10)
Supplement: Supplementary file 1 [file supplementary.tex]

% Compile this file to generate the supplementary PDF.
% In Overleaf, set supplementary.tex as the Main document for the supplementary material.
\def\SUPPLEMENTONLY{1}
\input{main.tex}
